# Supplementary material for: Towards a new social laboratory: An experimental study of search through community participation at Burning Man
Source: arXiv:1903.04125 source file (2019-03-11)
Supplement: Supplementary file 1 [file burning_man_SI.pdf]

# Towards a new social laboratory: An experimental study of search through community participation at Burning Man

Ziv Epstein[1*], Micah Epstein[2], Christian Almenar[3], Matt Groh[1], Niccolo Pescetelli[1], Esteban Moro[1,4], Manuel Cebrian[1], Nick Obradovich[1], and Iyad Rahwan[1]

[1]MIT Media Lab
[2]Rhode Island School of Design
[3]Intrinsic
[4]GISC & Universidad Carlos III de Madrid, Spain

March 11, 2019

## Supplemental information

### Scroll Text

All the text included in the scroll is as follows:

> **Preface**
> As a cartographer, we are asking that you help to contribute to the Black Rock Atlas, a community-driven art project and MIT research study.
> Burning Man is a magical place that allows our most creative and collaborative nature to flourish. Our goal is to understand the social systems that makes that magic possible. To do this, we are evolving the famous Six Degrees of Separation experiment and adapting it to the Playa. This vessel that was handed to you is intended to reach a final person (Terminus) while collecting images and GPS data. we kindly ask you to help us get it to them. If you are willing, please read the contents of this scroll, including the disclaimer (Specifications), and carry out the instructions to the right.
> **Terminus**
> With your help, this Vessel will make its way to this person, mapping its journey along the way.
> Playaname Playaname (a.k.a. Firstname Lastname) Origin: Cityname, Countryname Residence : Cityname, Countryname In one sentence and without mentioning your camp location, how might one find you
> **Cartography**
> To contribute to the Black Rock Atlas, we ask that you do the following:

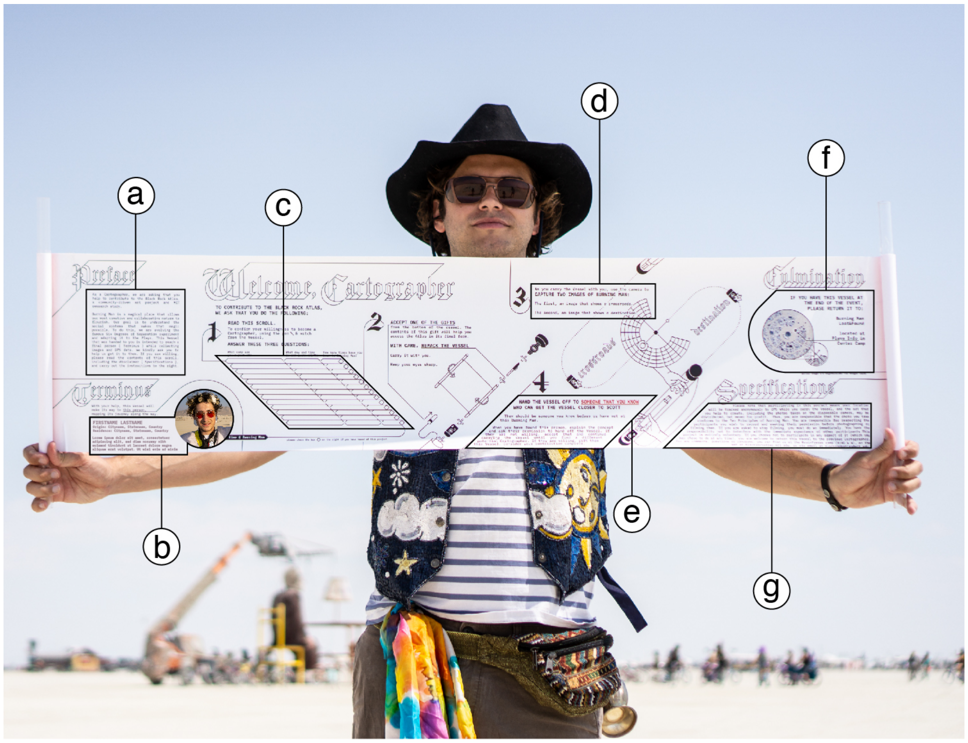


Figure 1: **The scroll.** Contains informed consent context (a), Terminus information (b), table for informed consent affirmation and hand-off time entry (c), instructions for photography (d), specific hand-off procedure (e), drop-off location if the event ends (f), and necessary disclosures and contact information (g).

1). Read this scroll. To confirm your willingness to become a cartographer, use a pen from the vessel to answer these three questions.
What camp are you part of?
What is the time and date? (with AM / PM)
How many times have you been to Burning Man?
2). Accept one of the gifts from the lid of the vessel. The contents of this gift will help you access the Atlas in its final form after the Burn.
With care, repack the Vessel.
Welcome, Cartographer. Carry it with you. Keep your eyes sharp.
3). As you carry the Vessel with you, use the camera to capture two images of Burning Man. The first, an image that shows a barrier. The second, an image that shows a destination.
6). Hand the Vessel off to someone that can get the vessel closer to the final person. They should be someone you knew before or have met at this Burning Man. When you have found this person, explain the concept and ask their permission to hand off the Vessel. If they are not willing, accept

that and continue carrying the Vessel until you find a different potential cartographer. If they are willing, gift them this Vessel. Consider your contribution complete

**Culmination**
If you have this Vessel at the end of the event, please return it to the Burning Man Lost and Found, located at Playa Info at Center Camp.

**Specifications**
Please note that participating in this project means your location will be tracked anonymously by GPS while you carry the vessel, and the art that you help to create, including the photos taken on the disposable camera, may be distributed, but never for profit. Thus, you are responsible that the photo you take conforms to the Ten Principles of Burning Man. You are responsible for respecting the participants you wish to record and seeking their permission before photographing or filming them. If you are asked to stop filming, you must do so immediately. You have the responsibility not to interfere with the immediate experience of other participants.This project is entirely voluntary. If you choose not to participate in any aspect of it (which you may chose to do at any time), you are welcome to return this vessel to the previous cartographer. For any comments, questions or concerns, you can find us at the BrainFreeze camp (4:45 & A), on the web at blackrockatlas.mit.edu, or via email at blackrockatlas@mit.edu."
